# Supplementary material for: A Multi-Layered Approach for Measuring the Simulation-to-Reality Gap of Radar Perception for Autonomous Driving
Source: arXiv:2106.08372 source file (2021-06-20)
Supplement: Supplementary file 1 [file 06_appendix.tex]

\section*{APPENDIX}
\label{appendix}
